# Supplementary material for: MEMOREPAIR: Barrier-First Cascade Repair in Agentic Memory
Source: arXiv:2605.07242 source file (2026-05-08)
Supplement: Supplementary file 1 [file appendix.tex]

\clearpage
\newpage
\appendix

\addcontentsline{toc}{part}{Appendix} 
\etocsettocstyle{\section*{Appendix Contents}}{} 
\etocsetnexttocdepth{subsection} 
\localtableofcontents
\bigskip

\newpage
\section{Notation}
\label{app:notation}

\begin{table}[h]
\centering
\footnotesize
\setlength{\tabcolsep}{4pt}

\begin{tabular}{@{}p{0.30\linewidth}p{0.64\linewidth}@{}}
\toprule
\textbf{Symbol} & \textbf{Meaning} \\
\midrule

$\mathcal{G}=(V,E^{\mathrm{inf}},E^{\mathrm{sem}})$
& Artifact graph with influence edges for repair scope and semantic edges for retrieval. \\

$(u,v)\in E^{\mathrm{inf}}$
& Artifact $v$ was produced using artifact $u$ as causal support. \\

$e=(F,\tau,\Delta)$
& Repair event with invalidated roots $F$, update type
$\tau\in\{\mathsf{delete},\mathsf{correct},\mathsf{migrate}\}$, and update data $\Delta$. \\

$X_\Delta$
& Fresh replacement artifacts materialized for correction events. \\

$C(F),D(F)$
& Affected cascade $\mathrm{Reach}(F;E^{\mathrm{inf}})$ and descendants $C(F)\setminus F$;
$\mathrm{Reach}$ includes the zero-hop roots in $F$. \\

$\kappa_e,\mathsf{Ret}(e)$
& Post-event interface and retained valid support in the post-event artifact universe. \\

$B_\rho$
& Hidden set for repair plan $\rho$, initialized to $C(F)$. \\

$\Phi_\mu^e$
& Event-indexed mode map assigning each affected descendant a mode in
$\{\mathsf{remove},\mathsf{recompute},\mathsf{regen},\mathsf{param}\}$. \\

$\mu_i$
& Repair mode assigned to descendant $i$. \\

$\Psi_e(i)=q_i$
& Graph-to-contract map returning
$q_i=(\mu_i,\pi_i,P_i,v_i,w_i,c_i)$. \\

$\pi_i$
& Repair operator for candidate $q_i$. \\

$P_i$
& Affected descendants whose repaired successors are consumed by $\pi_i$;
root replacements and interface updates are supplied through
$\mathsf{Ret}(e)$ and $\kappa_e$, not through $P_i$. \\

$D^+(F)$
& Non-removed candidate index set
$\{i\in D(F):\mu_i\neq\mathsf{remove}\}$. \\

$\bar P_i$
& Repairable required predecessors, $\bar P_i=P_i\cap D^+(F)$. \\

$v_i,w_i,c_i$
& Executability flag, candidate value, and normalized repair-operator cost. \\

$v_i^{(0)},\mathcal E_0$
& Initial executability flag before validation retry, and initially executable set
$\mathcal E_0=\{i\in D^+(F):v_i^{(0)}=1\}$. \\

$Q_\rho$
& Candidate family for repair plan $\rho$, $Q_\rho=\{q_i:i\in D^+(F)\}$. \\

$E^{\mathrm{req}}$
& Repair-dependency graph;
$(j,i)\in E^{\mathrm{req}}$ iff $j\in\bar P_i$, meaning $j$ must be staged before repairing $i$. \\

$z_i$
& Fresh successor version constructed for withdrawn artifact $i$. \\

$\mathrm{Validate}_i(z_i)$
& Validation oracle for successor $z_i$. \\

$\mathcal S_i,\mathrm{Prov}(z)$
& Neural-skill support multiset and artifact provenance of support example $z$. \\

$\mathsf{For}_i(e),\mathsf{New}_i(e),\mathsf{Ref}_i(e)$
& Invalidated, replacement, and retained reference support for parametric repair. \\

$\rho=(B_\rho,Q_\rho,S_\rho,R_\rho)$
& Repair plan: hidden set, candidate family, selected set, and republished successors. \\

$S_\rho,R_\rho$
& Selected candidate set and validated republished successor set. \\

$x_i,\lambda$
& Binary selection variable and repair--cost tradeoff parameter. \\

$\mathrm{Repair}(x),\mathrm{Cost}(x)$
& Scalarized objective terms:
$\mathrm{Repair}(x)=\sum_{i\in D^+(F)}w_i x_i$ and
$\mathrm{Cost}(x)=\sum_{i\in D^+(F)}c_i x_i$.\\

% $\mathrm{Cost}_{\mathrm{exec}}(\rho)$ &
% Reported realized normalized repair-operator Cost:
% $\mathrm{Cost}_{\mathrm{exec}}(\rho)=\sum_{i\in \Aexec} c_i$. \\
\bottomrule
\end{tabular}
\caption{Notation used in \textsc{MemoRepair}.}
\label{tab:notation-app}
\end{table}

\newpage
\section{Additional Experiments and Implementation Details}
\label{app:supplementary}

\subsection{Reproducibility Details}
\label{app:reproducibility}

\subsubsection{Hardware and Software}
\label{app:hardware-software}

All experiments are conducted on a single Ubuntu 22.04 server with
Python 3.12, PyTorch 2.8.0, and CUDA 12.8, equipped with
4$\times$ NVIDIA RTX 4090D, 18 vCPUs (AMD EPYC 9754), 128~GB RAM, and
a 500~GB SSD. Two base models are loaded locally through
\texttt{transformers}/\texttt{peft}/\texttt{bitsandbytes} under 4-bit
NF4 quantisation (bf16 compute, double quant): \textsc{LLaMA-7B}
(\texttt{huggyllama/llama-7b}) for parameter-level operator
experiments on the released \textsc{ToolLLaMA-7b-LoRA-v1} adapter,
and \textsc{Llama-3-8B-Instruct} for the cascade-side LoRA fine-tune
ablation. Both fit alongside their trainable LoRA adapter on a single
24~GB device. The 120B teacher
(\textsc{GPT-OSS-120B}), used for the prompt- and chain-repair stages
and as the validator backbone, is served via an OpenAI-compatible
\texttt{/chat/completions} endpoint with temperature~$0$ for
deterministic generation.

\subsubsection{Dataset Statistics}
\label{app:dataset-stats}

We use the public ToolBench and MemoryArena releases. From ToolBench we
draw all queries in groups G1, G2, and G3, which correspond to
single-tool, intra-category, and intra-collection multi-tool tasks
respectively. For the neural-skill stage we load up to $120$ queries
per skill, aggregate them by tool family, and keep the top three
families by frequency. Each query produces one ChatML
\texttt{(system, user, assistant)} triple from the first
\texttt{function\_call} in its answer trace; we use a stratified
val/train split with seed~$42$ (typically $0.20$/$0.80$, raised to
$0.25$/$0.75$ when per-skill data falls below the validation-coverage
threshold). The artifact-kind
distribution follows the four-way taxonomy of
Section~\ref{subsec:problem-setup}
(\texttt{record}, \texttt{cache}, \texttt{summary}, \texttt{skill}),
with \texttt{skill}s further partitioned into
\texttt{neural}/\texttt{prompt}/\texttt{chain}. In our cascade
statistics and case studies we aggregate \texttt{record},
\texttt{cache}, and \texttt{summary} into the operational
\texttt{CACHE} bucket and report \texttt{skill} separately, mirroring
the artifact-kind columns of Tables~\ref{tab:ma-deletion-anatomy}
and~\ref{tab:internal_main}. The chain-skill stage
cycles three migration scenarios
(\textit{nested-to-flat}, \textit{field-rename}, \textit{auth-change}).
MemoryArena cascades use the same projection and include $\mathsf{migrate}$ events, where the post-event interface $\kappa_e$ is updated and migrated successors are exposed to the validation oracle. MemoryArena draws from all five public subsets (\texttt{bundled\_shopping}, \texttt{progressive\_search}, \texttt{group\_travel\_planner}, \texttt{formal\_reasoning\_math}, \texttt{formal\_reasoning\_phys}) for a total of $701$ tasks.

Table~\ref{tab:cascade-stats} reports per-event sizes for the
invalidated root set $F$, the affected cascade $C(F)$, and the
repairable descendant set $D^{+}(F)$, together with the number of
events evaluated per benchmark and event type. Ranges are min--max
across events.

\begin{table}[!ht]
\centering\footnotesize
\setlength{\tabcolsep}{4.5pt}

\begin{tabular}{llcccc}
\toprule
\textbf{Benchmark} & \textbf{Event} &
$|F|$ & $|C(F)|$ & $|D^{+}(F)|$ & \textbf{\# events} \\
\midrule
\multirow{3}{*}{ToolBench}
& Deletion    & 1--8  & 12--128 & 9--96   & 276 \\
& Correction  & 1--6  & 10--112 & 8--84   & 276 \\
& Migration   & 1--5  & 14--124 & 11--94  & 276 \\
\midrule
\multirow{3}{*}{MemoryArena}
& Deletion    & 1--6  & 5--118  & 0--95   & 701 \\
& Correction  & 1--5  & 8--58   & 6--42   & 701 \\
& Migration   & 1--4  & 10--66  & 8--48   & 701 \\
\bottomrule
\end{tabular}
\caption{Per-event cascade statistics (min--max ranges).
MemoryArena Deletion is heavy-tailed: its $|D^{+}(F)|$ upper bound is
set by \texttt{progressive\_search} events.}
\label{tab:cascade-stats}
\end{table}

\subsubsection{Hyperparameters}
\label{app:hyperparameters}

\textbf{Repair tradeoff.}
The cost-aware selector uses $\lambda=0.3$ as the default tradeoff.
The Pareto sweep in Section~\ref{sec:experiment} covers
$\lambda \in \{0.1, 0.3, 1, 3, 10, 30\}$, plus the two endpoints
\emph{Remove all} ($\lambda \to \infty$) and \emph{Repair all}
($\lambda = 0$).

\textbf{LoRA fine-tune.}
The neural-skill stage uses two base models, one per experiment
stage. \emph{Operator-side experiments}
(Table~\ref{tab:parametric_operators}) run parameter-level repair
operators on the released \textsc{ToolBench/ToolLLaMA-7b-LoRA-v1}
adapter, which is itself a LoRA fine-tune of
\textsc{huggyllama/llama-7b}; we therefore load
\textsc{LLaMA-7B} as the base model for these runs to match the
released adapter's architecture. \emph{Cascade-side LoRA training}
(Figure~\ref{fig:parametric_pipeline} and the per-skill ablation
runs) trains fresh LoRA adapters on
\textsc{Llama-3-8B-Instruct} from the per-skill retain/forget
partitions; no cross-base adapter transfer is performed.
LoRA rank $r=8$, $\alpha=16$, dropout $0.05$, target modules
$\{\mathrm{q\_proj}, \mathrm{k\_proj}, \mathrm{v\_proj},
\mathrm{o\_proj}\}$. Optimization uses AdamW with $\text{lr}=10^{-4}$,
weight decay $0$, gradient clip $1.0$, and a cosine schedule with
$20$ warmup steps; batch size $16$, gradient accumulation $1$, and at
most $200$ steps with early stopping on validation loss (evaluated
every $25$ steps, patience $3$). Sequences are truncated at $2048$
tokens. Each per-skill seed is offset to $42 + i$ where $i$ indexes
the skill. Statistical variation in
Section~\ref{app:std-tables} is reported over global seeds
$\{42, 43, 44\}$, applied uniformly to data sampling, optimizer
state, and operator initialisation.

\textbf{Operator-side hyperparameters.}
All operators share the same training budget: at most $80$ steps,
batch size $4$, $\text{lr}=5\times 10^{-5}$, AdamW, gradient clip
$1.0$, sequence length $1024$, and 4-bit NF4 quantisation with bf16
compute and double-quant. The reference wall time for relative
compute is $120$~seconds (LUNE), so LUNE has relative compute $1.0$
by construction and the others are reported as
$\text{wall}/120\,\mathrm{s}$; LUNE serves only as the relative-compute
reference and is not tuned to favor \textsc{MemoRepair}.

\paragraph{Operator settings.}
For fairness, all parameter-level operators use the same training
budget and optimization setup. Operator-specific hyperparameters are
fixed globally across datasets, events, and seeds, with no per-event
tuning. For operators with recommended settings in prior work we
follow the corresponding default configuration; otherwise we choose
from a small held-out grid over the neural-skill validation split and
then freeze the selected configuration for all reported results. The
grids are $\beta\in\{0.05,0.1,0.2\}$ for NPO/SimNPO,
$\lambda_{\text{retain}}\in\{0.5,1.0,2.0\}$, RMU layer
$\in\{8,16,24\}$ with $c,\alpha\in\{0.5,1.0,2.0\}$, and the
forget/retain weights for BLUR, LUNE, and OOO in $\{0.5,1.0,2.0\}$.
SBU uses a two-phase suppress-then-boost split under the shared step
budget, and Full retrain runs the LoRA fine-tune defaults on the
retain partition.

\paragraph{Validation thresholds.}
Schema, safety, and sandbox checks are pass/fail. Task regression
requires every held-out probe to pass. Param-mode republication uses
$\tau_{\mathrm{FSP}}=\tau_{\mathrm{RU}}=80$. For reporting,
$\mathrm{ValPass}\%$ is the percentage of evaluated parametric successors
satisfying both $\mathrm{FSP}\ge80$ and $\mathrm{RU}\ge80$.

\subsubsection{Metrics}
\label{app:metric-details}

For each benchmark--event cell, Rep.\% is computed as
$
100\cdot
\frac{\sum_{e\in\mathcal{E}} |R_{\rho,e}|}
     {\sum_{e\in\mathcal{E}} |D^+_e(F)|}.
$
Events with $D^+_e(F)=\emptyset$ contribute zero to both sums. If the aggregate
denominator is zero, we report Rep.\ $=0$ and treat the cell as having no
publication opportunity. The denominator $D^+(F)$ contains all non-remove
repair contracts, including candidates that are statically non-executable after
candidate construction. A candidate enters $R_{\rho,e}$ only after its successor
passes the applicable validation checks. Thus \emph{Repair all} is an
executability-and-validation publication ceiling, not a $100\%$ publication
baseline.

For Cost, each candidate cost $c_i$ is normalized against the initially
executable set $E_0=\{i\in D^+(F):v_i^{(0)}=1\}$, following
Appendix~\ref{app:candidate-instantiation}. If $E_0=\emptyset$, no repair
operator is executed and the reported Cost is $0$. Otherwise, reported Cost
sums $c_i$ over executed repair operators, including attempts whose outputs
later fail validation; statically non-executable candidates and the withdrawal
barrier are not charged.

Leak\% and Stale-use\% are measured after the repair plan completes unless
otherwise stated. The withdrawal ablation in Table~\ref{tab:ablations} reports
repair-interval exposure, and the validation rows report validation false-pass
rates rather than post-repair action-level stale use.

For $\Delta$Task, $U_t$ denotes affected artifacts without a validated
republished successor, and $L_t$ denotes affected artifacts whose stale version
remains visible to task $t$. These sets may overlap: \emph{No action} can incur
both the missing-repair penalty and the stale-serving penalty, while
\emph{Remove all} incurs only the missing-repair penalty. For neural skills,
FSP and RU follow Appendix~\ref{app:validation-details}: if $a_i^F$ and $a_i^R$
are next-token accuracies reported in percentage points on the forget and
retain splits, then $\mathrm{FSP}_i=100-a_i^F$ and $\mathrm{RU}_i=a_i^R$. A
parametric successor passes validation when both exceed the fixed thresholds.

% ----------------------------------------------------------------
\subsection{Statistical Variation}
\label{app:std-tables}

Tables~\ref{tab:internal_std} and~\ref{tab:external_std} repeat
Tables~\ref{tab:internal_main} and~\ref{tab:external_main} of the main
paper, reporting each cell as mean~$\pm$~std over three seeds. Means
coincide with the main-paper values.

% Compact mean ± std cell: mean at normal size, ±std small and tucked to the right.
\providecommand{\msd}[2]{#1\,\raisebox{-0.25ex}{\tiny$\pm$#2}}

\begin{table}[!ht]
    \centering\footnotesize
    \setlength{\tabcolsep}{3pt}
    \begin{tabular}{l@{\hskip 3pt}rrr@{\hskip 6pt}rrr@{\hskip 6pt}rrr}
    \toprule
    \multirow{2}{*}{\textbf{Method}} &
    \multicolumn{3}{c}{\textbf{Deletion}} &
    \multicolumn{3}{c}{\textbf{Correction}} &
    \multicolumn{3}{c}{\textbf{Migration}} \\
    \cmidrule(lr){2-4}\cmidrule(lr){5-7}\cmidrule(lr){8-10}
    & Rep. & Cost & $\Delta$Task
    & Rep. & Cost & $\Delta$Task
    & Rep. & Cost & $\Delta$Task \\
    \midrule
    \multicolumn{10}{c}{\textbf{\textit{ToolBench}}} \\
    \midrule
    No action
    & -- & -- & \msd{$\text{-}2.78$}{0.12}
    & -- & -- & \msd{$\text{-}2.78$}{0.12}
    & -- & -- & \msd{$\text{-}5.61$}{0.21} \\

    \rowcolor{gray!12} Remove all
    & \msd{0.0}{0} & \msd{0.00}{0} & \msd{$\text{-}1.96$}{0.09}
    & \msd{0.0}{0} & \msd{0.00}{0} & \msd{$\text{-}1.96$}{0.09}
    & \msd{0.0}{0} & \msd{0.00}{0} & \msd{$\text{-}4.47$}{0.16} \\

    Repair all
    & \msd{24.6}{1.1} & \msd{1.00}{0} & \msd{$\text{-}1.54$}{0.06}
    & \msd{48.8}{1.4} & \msd{1.00}{0} & \msd{$\text{-}1.05$}{0.08}
    & \msd{38.7}{1.7} & \msd{1.00}{0} & \msd{$\text{-}2.98$}{0.13} \\

    \rowcolor{gray!12} Barrier+Greedy
    & \msd{20.3}{1.3} & \msd{0.72}{0.05} & \msd{$\text{-}1.68$}{0.09}
    & \msd{41.2}{2.0} & \msd{0.62}{0.04} & \msd{$\text{-}1.20$}{0.06}
    & \msd{31.4}{1.4} & \msd{0.76}{0.06} & \msd{$\text{-}3.28$}{0.15} \\

    \rowcolor{blue!10} \textsc{MemoRepair}
    & \msd{22.4}{0.9} & \msd{0.61}{0.04} & \msd{$\text{-}1.60$}{0.08}
    & \msd{45.1}{1.7} & \msd{0.57}{0.02} & \msd{$\text{-}1.11$}{0.05}
    & \msd{36.5}{1.1} & \msd{0.66}{0.05} & \msd{$\text{-}3.06$}{0.12} \\

    \midrule
    \multicolumn{10}{c}{\textbf{\textit{MemoryArena}}} \\
    \midrule
    No action
    & -- & -- & \msd{$\text{-}4.44$}{0.17}
    & -- & -- & \msd{$\text{-}4.44$}{0.17}
    & -- & -- & \msd{$\text{-}3.86$}{0.17} \\

    \rowcolor{gray!12} Remove all
    & \msd{0.0}{0} & \msd{0.00}{0} & \msd{$\text{-}4.00$}{0.15}
    & \msd{0.0}{0} & \msd{0.00}{0} & \msd{$\text{-}4.00$}{0.15}
    & \msd{0.0}{0} & \msd{0.00}{0} & \msd{$\text{-}3.58$}{0.12} \\

    Repair all
    & \msd{5.5}{0.9} & \msd{1.00}{0} & \msd{$\text{-}3.74$}{0.18}
    & \msd{35.6}{2.2} & \msd{1.00}{0} & \msd{$\text{-}2.91$}{0.13}
    & \msd{18.4}{1.4} & \msd{1.00}{0} & \msd{$\text{-}3.18$}{0.10} \\

    \rowcolor{gray!12} Barrier+Greedy
    & \msd{4.2}{1.0} & \msd{0.70}{0.08} & \msd{$\text{-}3.90$}{0.17}
    & \msd{28.6}{1.9} & \msd{0.83}{0.06} & \msd{$\text{-}3.17$}{0.15}
    & \msd{14.2}{1.5} & \msd{0.71}{0.04} & \msd{$\text{-}3.34$}{0.14} \\

    \rowcolor{blue!10} \textsc{MemoRepair}
    & \msd{5.1}{0.7} & \msd{0.62}{0.06} & \msd{$\text{-}3.79$}{0.16}
    & \msd{33.1}{1.8} & \msd{0.76}{0.05} & \msd{$\text{-}2.98$}{0.12}
    & \msd{17.0}{1.2} & \msd{0.64}{0.06} & \msd{$\text{-}3.23$}{0.11} \\

    \bottomrule
    \end{tabular}
    \caption{Repair-policy comparison with per-cell mean$\pm$std over
    three seeds; means coincide with Table~\ref{tab:internal_main}.
    Leak\,\%\ and Stale\,\%\ are omitted (constant by construction).}
    \label{tab:internal_std}
\end{table}

  \begin{table}[!ht]
    \centering\footnotesize
    \setlength{\tabcolsep}{4pt}
    \begin{tabular}{l@{\hskip 3pt}rrr@{\hskip 6pt}rrr@{\hskip 6pt}rrr}
    \toprule
    \multirow{2}{*}{\textbf{System}} &
    \multicolumn{3}{c}{\textbf{Deletion}} &
    \multicolumn{3}{c}{\textbf{Correction}} &
    \multicolumn{3}{c}{\textbf{Migration}} \\
    \cmidrule(lr){2-4}\cmidrule(lr){5-7}\cmidrule(lr){8-10}
    & Leak & Stale & $\Delta$Task
    & Leak & Stale & $\Delta$Task
    & Leak & Stale & $\Delta$Task \\
    \midrule
    \multicolumn{10}{c}{\textbf{\textit{ToolBench}}} \\
    \midrule
    No action
    & \msd{100}{0} & \msd{100}{0} & \msd{$\text{-}2.78$}{0.12}
    & \msd{100}{0} & \msd{100}{0} & \msd{$\text{-}2.78$}{0.12}
    & \msd{100}{0} & \msd{100}{0} & \msd{$\text{-}5.61$}{0.21} \\

    \rowcolor{gray!12} Mem0
    & \msd{74.6}{1.8} & \msd{93.8}{0.9} & \msd{$\text{-}2.61$}{0.10}
    & \msd{80.2}{1.5} & \msd{95.6}{0.7} & \msd{$\text{-}2.66$}{0.12}
    & \msd{91.3}{0.9} & \msd{98.9}{0.4} & \msd{$\text{-}5.46$}{0.19} \\

    Zep/Graphiti
    & \msd{69.8}{2.0} & \msd{92.4}{1.1} & \msd{$\text{-}2.54$}{0.11}
    & \msd{76.5}{1.7} & \msd{94.1}{0.8} & \msd{$\text{-}2.59$}{0.10}
    & \msd{89.1}{1.0} & \msd{98.4}{0.5} & \msd{$\text{-}5.39$}{0.18} \\

    \rowcolor{gray!12} MemR$^{3}$
    & \msd{85.2}{1.2} & \msd{98.6}{0.4} & \msd{$\text{-}2.72$}{0.08}
    & \msd{87.4}{1.0} & \msd{98.9}{0.3} & \msd{$\text{-}2.74$}{0.09}
    & \msd{92.6}{0.7} & \msd{99.6}{0.2} & \msd{$\text{-}5.48$}{0.16} \\

    A-MEM
    & \msd{72.1}{2.1} & \msd{92.7}{1.0} & \msd{$\text{-}2.56$}{0.12}
    & \msd{79.4}{1.6} & \msd{95.0}{0.7} & \msd{$\text{-}2.63$}{0.11}
    & \msd{90.6}{0.8} & \msd{98.7}{0.5} & \msd{$\text{-}5.42$}{0.18} \\

    \rowcolor{gray!12} O-Mem
    & \msd{88.7}{0.9} & \msd{99.4}{0.3} & \msd{$\text{-}2.73$}{0.08}
    & \msd{88.9}{0.8} & \msd{99.6}{0.2} & \msd{$\text{-}2.74$}{0.10}
    & \msd{93.1}{0.6} & \msd{99.7}{0.1} & \msd{$\text{-}5.51$}{0.17} \\

    TierMem
    & \msd{88.4}{1.0} & \msd{99.2}{0.4} & \msd{$\text{-}2.72$}{0.09}
    & \msd{88.6}{0.9} & \msd{99.5}{0.2} & \msd{$\text{-}2.74$}{0.08}
    & \msd{93.0}{0.5} & \msd{99.7}{0.1} & \msd{$\text{-}5.50$}{0.16} \\

    \rowcolor{blue!10} \textsc{MemoRepair}
    & \msd{0}{0} & \msd{0}{0} & \msd{$\text{-}1.60$}{0.08}
    & \msd{0}{0} & \msd{0}{0} & \msd{$\text{-}1.11$}{0.05}
    & \msd{0}{0} & \msd{0}{0} & \msd{$\text{-}3.06$}{0.12} \\

    \midrule
    \multicolumn{10}{c}{\textbf{\textit{MemoryArena}}} \\
    \midrule
    No action
    & \msd{100}{0} & \msd{100}{0} & \msd{$\text{-}4.44$}{0.17}
    & \msd{100}{0} & \msd{100}{0} & \msd{$\text{-}4.44$}{0.17}
    & \msd{100}{0} & \msd{100}{0} & \msd{$\text{-}3.86$}{0.17} \\

    \rowcolor{gray!12} Mem0
    & \msd{78.6}{2.3} & \msd{94.8}{1.0} & \msd{$\text{-}4.31$}{0.17}
    & \msd{82.4}{1.9} & \msd{96.1}{0.8} & \msd{$\text{-}4.18$}{0.15}
    & \msd{91.7}{1.1} & \msd{98.0}{0.6} & \msd{$\text{-}3.72$}{0.14} \\

    Zep/Graphiti
    & \msd{73.9}{2.5} & \msd{93.2}{1.2} & \msd{$\text{-}4.25$}{0.18}
    & \msd{78.1}{2.1} & \msd{94.6}{0.9} & \msd{$\text{-}4.07$}{0.16}
    & \msd{88.4}{1.3} & \msd{97.3}{0.7} & \msd{$\text{-}3.65$}{0.13} \\

    \rowcolor{gray!12} MemR$^{3}$
    & \msd{86.7}{1.4} & \msd{98.3}{0.5} & \msd{$\text{-}4.39$}{0.16}
    & \msd{88.2}{1.2} & \msd{98.7}{0.4} & \msd{$\text{-}4.31$}{0.15}
    & \msd{93.5}{0.9} & \msd{99.1}{0.3} & \msd{$\text{-}3.79$}{0.12} \\

    A-MEM
    & \msd{75.4}{2.2} & \msd{93.6}{1.1} & \msd{$\text{-}4.27$}{0.18}
    & \msd{80.3}{1.8} & \msd{95.2}{0.8} & \msd{$\text{-}4.12$}{0.16}
    & \msd{90.5}{1.2} & \msd{97.6}{0.6} & \msd{$\text{-}3.68$}{0.14} \\

    \rowcolor{gray!12} O-Mem
    & \msd{89.6}{1.0} & \msd{99.5}{0.3} & \msd{$\text{-}4.42$}{0.14}
    & \msd{90.1}{0.9} & \msd{99.6}{0.2} & \msd{$\text{-}4.36$}{0.13}
    & \msd{94.3}{0.7} & \msd{99.5}{0.2} & \msd{$\text{-}3.83$}{0.11} \\

    TierMem
    & \msd{89.2}{1.1} & \msd{99.3}{0.4} & \msd{$\text{-}4.41$}{0.15}
    & \msd{89.8}{0.9} & \msd{99.5}{0.3} & \msd{$\text{-}4.35$}{0.14}
    & \msd{93.9}{0.8} & \msd{99.4}{0.2} & \msd{$\text{-}3.82$}{0.12} \\

    \rowcolor{blue!10} \textsc{MemoRepair}
    & \msd{0}{0} & \msd{0}{0} & \msd{$\text{-}3.79$}{0.16}
    & \msd{0}{0} & \msd{0}{0} & \msd{$\text{-}2.98$}{0.12}
    & \msd{0}{0} & \msd{0}{0} & \msd{$\text{-}3.23$}{0.11} \\

    \bottomrule
    \end{tabular}
    \caption{Cascade-unaware comparison with per-cell mean$\pm$std
    over three seeds; means coincide with Table~\ref{tab:external_main}.
    Rep.\ and Cost\ are omitted (Rep.\,$=0$ and Cost\ undefined by
    construction).}
    \label{tab:external_std}
  \end{table}

% ----------------------------------------------------------------
\subsection{MemoryArena Deletion Cascade Anatomy}
\label{app:memoryarena-cascade-anatomy}

% To explain why MemoryArena deletion has the lowest Rep.\ ceiling
% ($5.5\%$) among the six (benchmark, event) combinations, we decompose
% the cascade $D^+(F)$ by \texttt{ArtifactKind} and tabulate, for each
% kind, how many descendants are structurally repairable under our
% operator set. Each kind defaults to a repair mode determined by how
% the artifact was produced: deterministic recomputations from a fixed
% input set (records, finals) default to \textsc{Exact}, while
% accumulative artifacts that aggregate support over time (skills)
% default to \textsc{Unlearn}. In this appendix, \textsc{Exact} denotes deterministic recomputation, and
% \textsc{Unlearn} denotes the parametric repair mode used for neural skills.

To explain why MemoryArena deletion has the lowest Rep.\ ceiling
($5.5\%$) among the six benchmark--event settings, we decompose
$D^+(F)$ by \texttt{ArtifactKind} and report which descendants are
structurally repairable. In this appendix, \textsc{Exact} denotes
deterministic recomputation, while \textsc{Unlearn} denotes parametric
repair for neural skills. Records and final answers default to
\textsc{Exact}; skills that aggregate support over time default to
\textsc{Unlearn}.

\begin{table}[!ht]
    \centering\footnotesize
    \setlength{\tabcolsep}{5pt}
    \begin{tabular}{lrrrl}
    \toprule
    \textbf{Kind} & $|D^+(F)|$ & \textbf{Republished} & \textbf{Rate} & \textbf{Dominant mode} \\
    \midrule
    \texttt{CACHE}\ (records, finals) & 160 & 0  & $0.0\%$  & \textsc{Exact}\,(missing parent) \\
    \texttt{SKILL}\ (memory\_skill)   & 22  & 10 & $45.5\%$ & \textsc{Unlearn} \\
    \midrule
    \textbf{Total}                    & \textbf{182} & \textbf{10} & $\mathbf{5.5\%}$ & -- \\
    \bottomrule
    \end{tabular}
    \caption{Per-kind anatomy of a single representative MemoryArena
    deletion event aggregated across the five subsets, not the
    event-level macro average underlying Tables~\ref{tab:internal_main}
    and~\ref{tab:cascade-stats}. Republished count is the number of
    validated successors under \emph{Repair all}.}
    \label{tab:ma-deletion-anatomy}
\end{table}

\paragraph{\texttt{CACHE} entries are structurally unrepairable.}
The 160 \texttt{CACHE} descendants, namely intermediate records and
final answers, are downstream products generated \emph{from} the
deleted artifact; recomputing them requires the deleted artifact as
input.
Once the parent is withdrawn, the recompute path is unavailable and
no \emph{validated} substitute is producible. Consequently every
\texttt{CACHE} candidate is quarantined at candidate-construction
time, and the Rep.\ contribution from this kind is \emph{exactly}
zero by structural argument, not by stochastic selector failure.

\paragraph{\texttt{SKILL} entries are repairable through
\textsc{Unlearn}.} The 22 \texttt{SKILL} descendants
(\texttt{memory\_skill} entries) use \textsc{Unlearn} as their
dominant mode: instead of recomputing from the deleted parent, the
operator emits a contract-restricted version that excises the deleted
support from the skill's retained reference set $\mathsf{Ref}_i(e)$.
Because \textsc{Unlearn} does not require the deleted parent to be
present, it sidesteps the structural infeasibility that defeats
\textsc{Exact} on \texttt{CACHE}. Of the 22 candidates, $10$ pass $\mathrm{Validate}_i$ on the
contract-restricted output, yielding a within-kind Rep.\ rate of
$45.5\%$. The remaining $12$ fail $\mathrm{Validate}_i$, indicating
that excising the deleted support degrades the skill below the
validator's coverage threshold; \textsc{MemoRepair} correctly retains
the withdrawal in this case rather than republishing a degraded
successor.

\paragraph{Aggregate ceiling.}
Weighting by cascade size, the deletion-cascade Rep.\ ceiling is
$10 / 182 \approx 5.5\%$, matching the \emph{Repair all} entry in
Table~\ref{tab:internal_main}. The headline rate is therefore not
evidence of repair-policy weakness; it reflects the structural
distribution of \texttt{ArtifactKind} in the cascade.
\textsc{MemoRepair} attains $5.1/5.5 \approx 93\%$ of this ceiling at
Cost $0.62$, matching the ceiling-recovery ratio it achieves on the
higher-Rep.\ MemoryArena correction and migration events.

\clearpage
% ----------------------------------------------------------------
  \newpage
  \section{Case Studies}
  \label{app:case-studies}

    To make the contract concrete, we walk through four local repair
    events from our evaluation: three successful repairs (a deletion
    on ToolBench, a correction on ToolBench, and a migration on
    MemoryArena) and one structural failure mode (a deletion on
    MemoryArena \texttt{progressive\_search}). Each case reports the
    event, the cascade structure, the per-descendant repair decision
    made by \textsc{MemoRepair}, and the outcome metrics.

  % ===== shared macros for case studies =====
  \definecolor{modecolor}{HTML}{2A4FA8}      % dark blue for mode names
  \definecolor{successgreen}{HTML}{2D7F4F}   % success
  \definecolor{failurered}{HTML}{C0392B}     % failure
  \newcommand{\mde}[1]{\textcolor{modecolor}{\textsc{#1}}}
  \newcommand{\tagsuccess}{\hfill\textcolor{successgreen}{\textbf{\checkmark\,Success}}}
  \newcommand{\tagfailure}{\hfill\textcolor{failurered}{\textbf{$\boldsymbol{\times}$\,Structural failure}}}

  % ----------------------------------------------------------------
  \subsection{\textcolor{blue}{Case 1: Deletion of a deprecated tool function (ToolBench)}}
  \label{app:case-deletion}

  \paragraph{Event.}
  The ToolBench finance tool \texttt{finnhub\_realtime\_stock\_price}
  (host \texttt{finnhub-realtime-stock-price.p.rapidapi.com}), with
  endpoints \texttt{Quote}, \texttt{Candles}, and
  \texttt{Stock\,Symbols}, is removed from the registry. We denote the
  removed tool by $f_{\text{quote}}$. The deletion event sets
  $F=\{f_{\text{quote}}\}$, no replacement artifact, and contract delta
  empty.

  \paragraph{Cascade ($|D^+(F)|=11$).}
  \begin{itemize}[leftmargin=*,itemsep=1pt]
  \item 4 cached \texttt{api\_call\_record} artifacts (responses to
  prior queries against the \texttt{Quote} and \texttt{Candles}
  endpoints).
  \item 3 derived summaries (\texttt{cached\_summary}) that aggregate
  the deleted tool's outputs together with two other tools.
  \item 1 prompt skill (\texttt{skill\_prompt}) for ``daily-market
  briefing''.
  \item 1 chain skill (\texttt{skill\_chain}) that calls
  \texttt{finnhub\_realtime\_stock\_price.Quote} as step~3 of a 5-step
  procedure.
  \item 2 neural skills (\texttt{skill\_neural}) trained on traces that
  include $f_{\text{quote}}$ outputs.
  \end{itemize}

  \paragraph{\textsc{MemoRepair} decisions.}
  \begin{itemize}[leftmargin=*,itemsep=1pt]
  \item 4 \texttt{api\_call\_record}s: quarantined under \mde{exact} mode
  (missing parent, no replacement) and withdrawn from service.
  \item 3 \texttt{cached\_summary}s: \mde{regen} executable using the
  remaining two tools' outputs as retained inputs; all 3 successors
  pass the validation oracle and re-enter service.
  \item 1 \texttt{skill\_prompt}: \mde{regen} against retained background
  context; passes validation; republished.
  \item 1 \texttt{skill\_chain}: rewritten by patching out step~3 and
  re-binding the downstream chain to a substitute tool; sandbox
  execution passes; republished.
  \item 2 \texttt{skill\_neural}s: \mde{unlearn} with non-empty forget /
  reference sets; both pass post-repair regression bound; republished.
  \end{itemize}

  \paragraph{Outcome.}
  $\text{Leak}=0$, $\text{Stale}=0$, $\text{Rep.}=63.6\%$
  (7 of 11 republished), $\text{Cost}=0.71$,
  $\Delta\text{Task}=-1.40$ (vs.\ $-2.78$ for No action and $-1.96$ for
  Remove all). Withdrawal alone closes the leak; min-cut selection
  keeps republication to validated successors. \tagsuccess

  % ----------------------------------------------------------------
  \subsection{\textcolor{blue}{Case 2: Correction of an API argument schema (ToolBench)}}
  \label{app:case-correction}

  \paragraph{Event.}
  The ToolBench travel tool \texttt{flight\_data\_v2} (host
  \texttt{travelpayouts-travelpayouts-flight-data-v1.p.rapidapi.com})
  corrects its \texttt{depart\_date} schema: the parameter, previously
  documented inconsistently across endpoints (variously
  \texttt{STRING}, \texttt{STRING (yyyy-mm)}, and
  \texttt{DATE\,(YYYY-MM-DD)} in the released tool spec), is normalized
  to ISO \texttt{YYYY-MM-DD} for all endpoints. We denote the
  corrected tool by $f_{\text{flight}}$. The correction event sets
  $F=\{f_{\text{flight}}\}$, \texttt{replacement\_artifact} = same
  kind/contexts/metadata as $f_{\text{flight}}$ with corrected version
  hash, and an empty contract delta.

  \paragraph{Cascade ($|D^+(F)|=8$).}
  \begin{itemize}[leftmargin=*,itemsep=1pt]
  \item 5 \texttt{api\_call\_record}s issued against
  \texttt{flight\_data\_v2} with the legacy non-ISO date format.
  \item 1 \texttt{cached\_summary} of recent flight queries.
  \item 1 \texttt{skill\_chain} that issues
  \texttt{depart\_date} arguments.
  \item 1 \texttt{skill\_neural} fine-tuned on flight planning traces.
  \end{itemize}

  \paragraph{\textsc{MemoRepair} decisions.}
  \begin{itemize}[leftmargin=*,itemsep=1pt]
  \item 5 \texttt{api\_call\_record}s: \mde{exact} recompute against the
  replacement (which carries the corrected schema). 4 of 5 are
  initially executable and succeed under the corrected schema; 1 has a
  retained \texttt{depart\_date} argument in a non-ISO custom locale
  that the replacement schema cannot interpret, fails the executability
  precheck ($v_i^{(0)}=0$), and is quarantined at candidate
  construction without invoking \mde{exact} recompute.
  \item 1 \texttt{cached\_summary}: \mde{regen} against the 4 successful
  records plus retained context; passes validation; republished.
  \item 1 \texttt{skill\_chain}: argument rebinding to ISO format;
  sandbox replay over 5 anchor calls returns matching outputs;
  republished.
  \item 1 \texttt{skill\_neural}: \mde{unlearn} with the legacy-format
  records as forget set, ISO records as reference; passes regression
  bound; republished.
  \end{itemize}

  \paragraph{Outcome.}
  $\text{Leak}=0$, $\text{Stale}=0$, $\text{Rep.}=87.5\%$
  (7 of 8 republished), $\text{Cost}=0.78$,
  $\Delta\text{Task}=-0.92$ (vs.\ $-2.78$ for No action and $-1.96$ for
  Remove all). The single barrier-side quarantine demonstrates that
  the executability precheck catches retained-input incompatibilities
  before \mde{exact} is invoked, so the operator cost is not charged
  for unrepairable candidates. \tagsuccess

  % ----------------------------------------------------------------
  \subsection{\textcolor{blue}{Case 3: Migration of an attribute schema (MemoryArena)}}
  \label{app:case-migration}

  \paragraph{Event.}
  In the MemoryArena \texttt{bundled\_shopping} subset, the
  \texttt{electronics\_item} category has its attribute schema
  migrated: free-form attribute strings (e.g.\ \texttt{``50-inch''},
  \texttt{``4K HD''}, \texttt{``LED screen''}) are normalized to
  structured key-value attributes (e.g.\
  \texttt{\{size:\,50-inch, resolution:\,4K, panel:\,LED\}}) under a
  new schema. We denote the migrated schema by $c_{\text{elec}}$. The
  migration event sets $F=\{c_{\text{elec}}\}$, no replacement
  artifact, and contract delta records the attribute schema rewrite.

  \paragraph{Cascade ($|D^+(F)|=14$).}
  \begin{itemize}[leftmargin=*,itemsep=1pt]
  \item 12 \texttt{api\_call\_record}s capturing webshop interactions
  whose product-selection answers carry legacy free-form attribute
  strings.
  \item 1 \texttt{cached\_result} (final consolidated bundle for the
  affected task).
  \item 1 \texttt{skill\_neural} (memory skill summarising
  electronics-bundle preferences across affected tasks).
  \end{itemize}

  \paragraph{\textsc{MemoRepair} decisions.}
  \begin{itemize}[leftmargin=*,itemsep=1pt]
  \item 12 \texttt{api\_call\_record}s: \mde{exact} recompute under
  the post-event migrated contract supplied through $\kappa_e$. 11 of
  12 are initially executable and re-derive their attribute lists into
  the structured key-value form with schema validation passing; one
  record contains a free-form attribute (\texttt{``smart TV''}) that
  has no canonical key under the migrated schema, fails the
  executability precheck ($v_i^{(0)}=0$), and is quarantined at
  candidate construction without invoking \mde{exact} recompute.
  \item 1 \texttt{cached\_result}: \mde{exact} recompute against the staged
  records; passes validation; republished.
  \item 1 \texttt{skill\_neural}: \mde{unlearn} with the
  legacy-contract view of the affected traces as forget set, and the
  remaining retained traces re-rendered under the post-migration
  contract $\kappa_e$ as reference. The reference set is the same
  $\mathsf{Ref}_i(e)=\mathcal S_i\setminus \mathsf{For}_i(e)$ from
  Section~\ref{subsec:problem-setup}; no new training examples are
  materialized. Passes regression and republished.
  \end{itemize}

  \paragraph{Outcome.}
  $\text{Leak}=0$, $\text{Stale}=0$, $\text{Rep.}=92.9\%$
  (13 of 14 republished), $\text{Cost}=0.69$,
  $\Delta\text{Task}=-2.05$ (vs.\ $-3.86$ for No action and $-3.58$ for
  Remove all).
  Migration retains the original artifact, which is why this case
  recovers $>90\%$ of the cascade; this contrasts with the
  deletion-on-MemoryArena setting where the deleted anchor provides
  no replacement and \mde{exact} recompute is structurally infeasible
  (Appendix~\ref{app:memoryarena-cascade-anatomy}). \tagsuccess

  % ----------------------------------------------------------------
  \subsection{\textcolor{red}{Case 4: Deletion with empty retained support — failure mode (MemoryArena
  \texttt{progressive\_search})}}
  \label{app:case-failure}

  \paragraph{Event.}
  On the MemoryArena \texttt{progressive\_search} subset, each task
  consists of $\sim$8 sequential subquestions that all resolve to a
  single anchor entity (e.g., the task at \texttt{id=0} chains nine
  biographical clues onto one named individual). The deletion event
  removes a foundational entity record $r_{\text{anchor}}$ that serves
  as this shared answer target across an affected task cluster. Every
  record in the chain is conditioned on $r_{\text{anchor}}$, and the
  neural memory skill is trained exclusively on traces that reference
  this entity. The deletion event sets $F=\{r_{\text{anchor}}\}$, no
  replacement artifact, and contract delta empty.

  \paragraph{Cascade ($|D^+(F)|=79$).}
  \begin{itemize}[leftmargin=*,itemsep=1pt]
  \item 63 \texttt{api\_call\_record}s recording every subquestion
  resolution in the affected cluster, each with $r_{\text{anchor}}$ as
  a load-bearing parent.
  \item 8 \texttt{cached\_result}s (per-task final consolidated
  answers).
  \item 8 \texttt{skill\_neural}s (memory skills fine-tuned exclusively
  on traces from these tasks).
  \end{itemize}

  \paragraph{\textsc{MemoRepair} decisions.}
  \begin{itemize}[leftmargin=*,itemsep=1pt]
  \item 63 \texttt{api\_call\_record}s: all 63 quarantined under \mde{exact}
  mode, since the deleted entity has no replacement and deterministic
  recompute cannot fabricate a missing answer target.
  \item 8 \texttt{cached\_result}s: all 8 quarantined because their staged
  record predecessors are themselves quarantined, so the staged-input
  check fails.
  \item 8 \texttt{skill\_neural}s: all 8 quarantined under the
  \emph{empty reference support} guard, since every retained training
  example referenced the deleted entity, leaving
  $\mathsf{Ref}_i(e)=\emptyset$, and the contract refuses to fit
  on an empty reference set.
  \end{itemize}

  \paragraph{Outcome.}
  $\text{Leak}=0$, $\text{Stale}=0$, $\text{Rep.}=0\%$
  (no validated successor publishable; all $79$ descendants are
  structurally quarantined), $\text{Cost}=0.00$,
  $\Delta\text{Task}=-4.00$ (vs.\ $-4.44$ for No action). Repair
  coverage collapses to zero, but withdrawal alone still recovers
  $0.44$ task points by preventing stale serving; the barrier-first
  contract continues to deliver its lower-bound guarantee even when
  the selector has nothing to publish. \tagfailure

  % ----------------------------------------------------------------
  \paragraph{Discussion.}
  Case~4 marks the structural boundary of the \textsc{MemoRepair}
  contract. The \texttt{progressive\_search} subset concentrates the
  entire retained training support of the neural skill inside the
  chain that the deleted entity anchors, so the deletion
  simultaneously (i)~removes the only parent of every cached record,
  making \mde{exact} infeasible without a replacement, and
  (ii)~empties the $\mathsf{Ref}_i(e)$ set of every neural skill,
  triggering \mde{unlearn}'s executability guard. No selector
  (repair-all, greedy, or min-cut) can publish a validated successor
  in this regime: the contract has no successor to publish. The
  contract's refusal to fabricate parents or fit on empty reference
  support is what prevents silent hallucination of repaired state.

  What \textsc{MemoRepair} provides here is the
  \emph{withdrawal lower bound}. The $0.44$-point $\Delta$Task gain
  over No action arises entirely from the barrier, with the selector
  inactive. This isolates a property of barrier-first design that is
  masked when withdrawal and selection both contribute: when nothing
  is republishable, the barrier still bounds downstream regression.
  Methods that conflate withdrawal with selection, for instance
  greedy without a withdrawal contract, cannot deliver this guarantee:
  they either leak stale records or fabricate replacements that fail
  validation. The per-kind breakdown in
  Appendix~\ref{app:memoryarena-cascade-anatomy} shows that
  \texttt{progressive\_search} is the unique MemoryArena subset where
  both \mde{exact} and \mde{unlearn} executability guards trigger
  simultaneously.

\newpage

\section{Provenance Projection and Repair Dependencies}
\label{app:provenance-details}

The implementation may record a finer-grained execution--artifact graph
\[
\mathcal{G}_{\mathrm{prov}}
=
(\mathcal{X}\cup\mathcal{A},E_{\mathrm{prov}}),
\]
where $\mathcal{X}$ denotes execution events and $\mathcal{A}$ denotes
artifact records. \textsc{MemoRepair} first projects this log onto durable
artifacts $V\subseteq\mathcal{A}$, yielding a raw artifact-level
influence graph
\[
\mathcal{G}_{\mathrm{raw}}
=
(V,E^{\mathrm{inf}}_{\mathrm{raw}},E^{\mathrm{sem}}).
\]
A raw influence edge $(u,v)\in E^{\mathrm{inf}}_{\mathrm{raw}}$ is added
when $\mathcal{G}_{\mathrm{prov}}$ contains evidence that artifact $v$
was produced using artifact $u$ as causal support. Semantic relations are
recorded separately in $E^{\mathrm{sem}}$ and do not enter cascade
localization.

Iterative memory updates can create cycles in
$E^{\mathrm{inf}}_{\mathrm{raw}}$. We therefore condense the strongly
connected components of $(V,E^{\mathrm{inf}}_{\mathrm{raw}})$ before
reachability is computed. Let
\[
\mathcal{H}
=
(V_{\mathrm{scc}},E^{\mathrm{inf}}_{\mathrm{scc}})
\]
be this SCC condensation, and let $[v]$ denote the SCC containing
artifact $v$. For a root set $F$, define
\[
[F]=\{[f]:f\in F\}.
\]
Cascade localization is computed on $\mathcal H$ and lifted back to
artifacts:
\[
C(F)
=
\bigcup_{S\in \mathrm{Reach}([F];E^{\mathrm{inf}}_{\mathrm{scc}})} S,
\qquad
D(F)=C(F)\setminus F .
\]
Thus an artifact is affected in the raw graph exactly when its SCC is
reachable from a root SCC in the condensed graph. In the main text, we
write this lifted operation compactly as
$\mathrm{Reach}(F;E^{\mathrm{inf}})$.

The repair-dependency graph $E^{\mathrm{req}}$ has a different meaning
from influence provenance. For a candidate $q_i$, the set
$P_i\subseteq D(F)$ contains only affected descendants whose repaired
successors are explicitly consumed by the repair operator $\pi_i$; root
replacements and interface updates are supplied through
$\mathsf{Ret}(e)$ and $\kappa_e$ rather than through $P_i$. The
repair-time dependency graph is
\[
E^{\mathrm{req}}
=
\{(j,i):i\in D^+(F),\,j\in P_i\cap D^+(F)\}.
\]
An edge $(j,i)\in E^{\mathrm{req}}$ states that the repaired successor of
$j$ must be staged before the successor of $i$ can be executed. Thus
$E^{\mathrm{req}}$ is induced by the local repair contracts
$\Psi_e(i)$, not by all provenance links.

\clearpage
\newpage

\section{Candidate Instantiation}
\label{app:candidate-instantiation}

\paragraph{Mode matching.}
The mode-assignment map $\Phi_\mu^e$ is deterministic. A neural skill
whose training support intersects $C(F)$ and admits nonempty
$(\mathsf{For}_i(e),\mathsf{Ref}_i(e))$ partitions is assigned
$\mathsf{param}$. A deterministic cache or materialized artifact with a
valid replay trace under $\kappa_e$ is assigned $\mathsf{recompute}$.
A summary, prompt skill, or chain procedure with sufficient retained
support is assigned $\mathsf{regen}$. If none of these conditions holds,
the artifact is assigned $\mathsf{remove}$. These rules are fixed across
events and benchmarks.

\paragraph{Predecessor requirements.}
For each candidate $q_i$, $P_i\subseteq D(F)$ contains only affected
descendants whose repaired successors are explicitly consumed by
$\pi_i$. Root replacements and interface updates are supplied through
$\mathsf{Ret}(e)$ and $\kappa_e$, not through $P_i$. For recomputation,
$P_i$ is read from the replay trace and restricted to affected
descendants. For regeneration, $P_i$ contains affected summaries, caches,
or procedure components used in the regeneration context. For
chain-skill regeneration, $P_i$ also includes affected API-contract or
cached-output descendants required by the sandbox harness. Semantic
retrieval edges are never included.

Let $v_i^{(0)}$ denote the executability flag after static candidate
filtering and before validation retry. Candidates with unavailable,
non-repairable, or cyclic requirements are assigned $v_i^{(0)}=0$.
Selection retries may later set $v_i\leftarrow0$ after validation
failure, but the normalized value and cost terms below remain fixed.

\paragraph{Cost and value.}
Let
\[
\mathcal E_0=\{i\in D^+(F):v_i^{(0)}=1\}
\]
be the initially executable candidate set. Candidate cost is the
normalized resource cost of its repair operator:
\[
\tilde c_i=
\alpha_{\mathrm{tool}}n_i^{\mathrm{tool}}
+\alpha_{\mathrm{tok}}n_i^{\mathrm{tok}}
+\alpha_{\mathrm{gpu}}t_i^{\mathrm{gpu}}
+\alpha_{\mathrm{sand}}t_i^{\mathrm{sand}},
\qquad
c_i=\frac{\tilde c_i}
{\sum_{j\in\mathcal E_0}\tilde c_j+\epsilon}.
\]
Here $n_i^{\mathrm{tool}}$ is the number of replayed tool calls,
$n_i^{\mathrm{tok}}$ is the number of LLM tokens used for regeneration,
$t_i^{\mathrm{gpu}}$ is GPU time for parametric repair, and
$t_i^{\mathrm{sand}}$ is sandbox execution time. The coefficients
$\alpha$ are fixed before evaluation.

Candidate value is a fixed trace-derived score:
\[
\tilde w_i=
\log(1+n_i^{\mathrm{use}})
+\log\!\left(
1+
\left|
(\mathrm{Reach}(i;E^{\mathrm{inf}})\setminus\{i\})\cap D(F)
\right|
\right)
+\frac{n_i^{\mathrm{probe}}}
{\max_{j\in\mathcal E_0} n_j^{\mathrm{probe}}+\epsilon}.
\]
For nondegenerate events,
\[
w_i=\frac{\tilde w_i}
{\sum_{j\in\mathcal E_0}\tilde w_j+\epsilon}.
\]
Here $n_i^{\mathrm{use}}$ counts historical retrieval or execution, the
reachability term measures affected downstream fan-out, and
$n_i^{\mathrm{probe}}$ counts held-out probes referencing $i$. If all
$\tilde w_j$ are zero over $\mathcal E_0$, we use uniform values over
$\mathcal E_0$.

\paragraph{Parametric support construction.}
For a neural skill $i$, let $\mathcal S_i$ denote the support multiset
used to train its current parameters, and let $\mathrm{Prov}(z)$ be the
artifact provenance of support example $z\in\mathcal S_i$. In the
notation of Section~\ref{subsec:problem-setup}, $\mathcal S_i$
corresponds to the training support set $D_i$; we use $\mathcal S_i$
here to emphasise that all operations below are multiset operations. We define
\[
\mathsf{For}_i(e)
=
\{z\in\mathcal S_i:\mathrm{Prov}(z)\cap C(F)\neq\varnothing\}.
\]
For correction events, replacement support is materialized from the
correction payload:
\[
\mathsf{New}_i(e)=
\begin{cases}
\mathrm{Materialize}(X_\Delta,i), & \tau=\mathsf{correct},\\
\varnothing, & \tau\in\{\mathsf{delete},\mathsf{migrate}\}.
\end{cases}
\]
The retained reference support is
\[
\mathsf{Ref}_i(e)
=
(\mathcal S_i\setminus \mathsf{For}_i(e))\cup \mathsf{New}_i(e).
\]
A parametric candidate is executable only when
$\mathsf{For}_i(e)$ and $\mathsf{Ref}_i(e)$ are both nonempty and the
chosen parameter-level repair operator can consume this pair.

\newpage
\section{Validation Oracle Implementation}
\label{app:validation-details}

The oracle $\mathrm{Validate}_i(z_i)\in\{0,1\}$ from
Section~\ref{subsec:withdrawal-barrier} runs three coverage levels:
\emph{schema-only}, \emph{task-regression-only}, and \emph{full}.
Main-paper experiments use \emph{full}; the other two appear only in the
validation-coverage ablation (Table~\ref{tab:ablations}).

\textbf{Cascade precheck.}
The oracle first rejects any successor whose declared parents intersect
the still-hidden cascade $B_\rho=C(F)$, except for fresh correction
replacements in $X_\Delta$. For $\mathsf{param}$ successors, it also
rejects any successor whose training support still references a hidden
artifact.

\textbf{Per-artifact checks.}
\emph{Schema} applies to $\mathsf{recompute}$ and $\mathsf{regen}$
successors, including regenerated chain skills. The rendered value must
contain every key in the artifact's declared required-output schema,
populated from the ToolBench tool contract or the MemoryArena structured
output schema. Successors with no declared schema skip the schema check
but must still pass all other applicable checks.

\emph{Task regression} replays held-out probes: $25\%$ of per-skill
ChatML triples for neural skills, held-out demonstrations for prompt
skills, and scenario inputs for chain skills. A probe passes when the
gold function name and all gold argument keys are present in the
prediction.

\emph{Safety} rejects values whose safety probe fails or that contain a
blocked output token, such as leaked legacy field names or stale OAuth
tokens. \emph{Sandbox} applies only to chain skills: it executes the
rewritten function in an isolated Python subprocess under a 5-second
timeout and requires every scenario input to return cleanly.

\textbf{Parametric checks.}
For $\mathsf{param}$ successors, let $a_i^F$ and $a_i^R$ be next-token
accuracy on the forget and retain splits of
$(\mathsf{For}_i(e),\mathsf{Ref}_i(e))$, masked at the prompt prefix. We
define
\[
\mathrm{FSP}_i=100-a_i^F,\qquad
\mathrm{RU}_i=a_i^R.
\]
A parametric successor passes validation when
\[
\mathrm{FSP}_i\ge\tau_{\mathrm{FSP}},
\qquad
\mathrm{RU}_i\ge\tau_{\mathrm{RU}},
\]
with $\tau_{\mathrm{FSP}}=\tau_{\mathrm{RU}}=80$. For reporting,
$\mathrm{ValPass}\%$ is the percentage of evaluated parametric
successors satisfying both thresholds.

\textbf{Composition and quarantine.}
Full validation requires all applicable checks to pass. A failed
candidate is not republished and is marked non-executable
($v_i\leftarrow0$). The selector is rerun on the updated candidate
family, which removes descendants requiring the failed candidate unless
they remain feasible through another predecessor-closed selection.
Candidates that remain unselected after the final iteration stay
withdrawn.
% ================================================================

\newpage

\section{Proof of Theorem~\ref{thm:cost-aware-repair}}
\label{app:proof-cost-aware-repair}

Fix a repair event $e$, a candidate family
$Q_\rho=\{q_i:i\in D^+(F)\}$, the current executability flags
$\{v_i\}$, and a tradeoff parameter $\lambda\ge0$. For each
$i\in D^+(F)$, let $x_i\in\{0,1\}$ indicate whether candidate $q_i$ is
selected. The scalarized repair-selection problem is
\[
\max_x
\sum_{i\in D^+(F)} w_i x_i
-
\lambda
\sum_{i\in D^+(F)} c_i x_i
\]
subject to
\[
x_i\le v_i,\qquad
x_i\le x_j\ \ \forall j\in \bar P_i,\qquad
x_i\in\{0,1\}.
\]
Here $\bar P_i=P_i\cap D^+(F)$ is the set of repairable required
predecessors. If $P_i\setminus D^+(F)\neq\varnothing$, then $i$ has a
non-repairable requirement and is encoded by setting $v_i=0$.

Define
\[
p_i \triangleq w_i-\lambda c_i .
\]
Then the objective becomes
\[
\max_x\ \sum_{i\in D^+(F)} p_i x_i .
\]
Let
\[
\mathcal V \triangleq D^+(F).
\]
For any feasible binary vector $x$, define
\[
U(x)\triangleq \{i\in\mathcal V:x_i=1\}.
\]
The constraints $x_i\le v_i$ imply
\[
U(x)\subseteq \mathcal V_{\mathrm{exec}},
\qquad
\mathcal V_{\mathrm{exec}}\triangleq\{i\in\mathcal V:v_i=1\}.
\]
The predecessor-closure constraints imply
\[
i\in U(x)\Longrightarrow \bar P_i\subseteq U(x).
\]
Therefore feasible selections are exactly the executable
predecessor-closed subsets $U\subseteq\mathcal V$, and the problem is
equivalent to
\[
\max_{U\subseteq\mathcal V}\ \sum_{i\in U}p_i
\]
subject to
\[
U\subseteq \mathcal V_{\mathrm{exec}},
\qquad
i\in U\Rightarrow \bar P_i\subseteq U.
\]

We now reduce this maximum-weight predecessor-closure problem to a
minimum $s$--$t$ cut. Construct a directed capacitated network with node
set
\[
\mathcal N\triangleq \{s,t\}\cup\mathcal V,
\]
where $s$ is the source and $t$ is the sink. For each $i\in\mathcal V$:
\begin{enumerate}[leftmargin=*,label=(\roman*)]
    \item if $p_i>0$, add an edge $s\to i$ with capacity $p_i$;
    \item if $p_i<0$, add an edge $i\to t$ with capacity $-p_i$;
    \item if $p_i=0$, add no reward edge incident to $i$.
\end{enumerate}
Let
\[
W^+\triangleq \sum_{i:p_i>0}p_i,
\qquad
M>W^+ .
\]
For every non-executable node $i$ with $v_i=0$, add an exclusion edge
$i\to t$ of capacity $M$. For every required predecessor
$j\in\bar P_i$, add a dependency edge $i\to j$ of capacity $M$.
Although $E^{\mathrm{req}}$ is oriented from prerequisite to dependent
for execution, these min-cut dependency edges are oriented from the
dependent to the prerequisite so that selecting $i$ forces selecting
$j$.

Now consider any $s$--$t$ cut $(S,T)$ with $s\in S$ and $t\in T$, and
define
\[
U(S)\triangleq S\cap\mathcal V .
\]
The contribution of positive-reward edges is
\[
\sum_{i:p_i>0,\ i\notin U(S)}p_i
=
W^+-
\sum_{i\in U(S),\,p_i>0}p_i.
\]
The contribution of negative-reward edges is
\[
\sum_{i:p_i<0,\ i\in U(S)}(-p_i).
\]
Combining these finite reward-edge contributions gives
\[
W^+-\sum_{i\in U(S)}p_i.
\]

If $U(S)$ contains a non-executable node $i$ with $v_i=0$, then the
exclusion edge $i\to t$ is cut and incurs capacity $M$. If $U(S)$
contains a node $i$ but omits a required predecessor $j\in\bar P_i$,
then the dependency edge $i\to j$ is cut and also incurs capacity $M$.
Thus
\[
\operatorname{Cap}(S,T)
=
W^+-\sum_{i\in U(S)}p_i
+
M\,N_{\mathrm{pen}}(S),
\]
where $N_{\mathrm{pen}}(S)$ is the number of cut $M$-capacity penalty
edges.

If $N_{\mathrm{pen}}(S)\ge1$, then
\[
\operatorname{Cap}(S,T)
\ge
W^+-\sum_{i\in U(S)}p_i+M.
\]
Since
\[
\sum_{i\in U(S)}p_i
\le
\sum_{i:p_i>0}p_i
=
W^+,
\]
we have
\[
\operatorname{Cap}(S,T)\ge M>W^+.
\]
The trivial cut
\[
S=\{s\},\qquad T=\mathcal N\setminus\{s\}
\]
has capacity exactly $W^+$, because it cuts only the edges $s\to i$ with
$p_i>0$. Hence any cut with a penalty edge cannot be minimum. Therefore
every minimum cut induces an executable predecessor-closed set $U(S)$.

For any cut with no penalty edge, we have
\[
\operatorname{Cap}(S,T)
=
W^+-\sum_{i\in U(S)}p_i.
\]
Since $W^+$ is constant, minimizing cut capacity is equivalent to
maximizing
\[
\sum_{i\in U(S)}p_i
=
\sum_{i\in U(S)}(w_i-\lambda c_i),
\]
which is exactly the scalarized repair objective.

Conversely, given any executable predecessor-closed subset
$U\subseteq\mathcal V$, define
\[
S(U)=\{s\}\cup U,
\qquad
T(U)=\mathcal N\setminus S(U).
\]
Because $U$ is feasible, no $M$-capacity penalty edge is cut, and the
resulting cut capacity is
\[
W^+-\sum_{i\in U}p_i.
\]
Thus feasible repair sets and cuts without penalty edges correspond up
to the constant offset $W^+$. Therefore a minimum $s$--$t$ cut yields an
optimal executable predecessor-closed repair set. This proves the
theorem.

\clearpage
\newpage

\section{Full execution algorithm}
\label{app:full-execution-algorithm}

Algorithm~\ref{alg:memo-repair-full} gives the full execution
procedure. Candidate construction is handled by the graph-to-contract
map $\Psi_e$ defined in Appendix~\ref{app:candidate-instantiation}. The
selection step runs on the full candidate family $Q_\rho$, including
non-executable candidates, so that closure constraints on their
dependents remain explicit.

\begin{algorithm}[!ht]
\caption{\textsc{MemoRepair} (full execution)}
\label{alg:memo-repair-full}
\begin{algorithmic}[1]
\REQUIRE Repair event $e=(F,\tau,\Delta)$, memory graph $\mathcal{G}$,
interface $\kappa$, acknowledgement timeout $T_{\mathrm{ack}}$, tradeoff parameter $\lambda$
\ENSURE Hidden set $B_\rho$, candidate family $Q_\rho$, selected set $S_\rho$, republished successors $R_\rho$

\STATE Compute post-event interface $\kappa_e$
\STATE Compute affected cascade $C(F)$, descendants $D(F)$, and retained support $\mathsf{Ret}(e)$
\STATE Set hidden set $B_\rho\leftarrow C(F)$ and enforce withdrawal barrier on $B_\rho$

\STATE Assign modes
$\mu_i=\Phi_\mu^e(i;\mathcal G,\mathsf{Ret}(e),\kappa_e)$ for all $i\in D(F)$
\STATE Set
\[
D^+(F)\leftarrow \{i\in D(F):\mu_i\neq\mathsf{remove}\}
\]
\STATE Build candidate family
\[
Q_\rho \leftarrow \{\Psi_e(i):i\in D^+(F)\}
\]
\STATE For each $q_i\in Q_\rho$, compute
\[
\bar P_i\leftarrow P_i\cap D^+(F).
\]
If $P_i\setminus D^+(F)\neq\varnothing$, set $v_i\leftarrow0$.
\STATE Build
\[
E^{\mathrm{req}}\leftarrow
\{(j,i):i\in D^+(F),\,j\in\bar P_i\}.
\]
\STATE Mark candidates in cyclic repair requirements non-executable
\STATE Initialize $R_\rho\leftarrow\varnothing$

\REPEAT
    \STATE Solve \eqref{eq:scalarized-selection}--\eqref{eq:binary} on $Q_\rho$ to obtain
    $S_\rho=\{i:x_i=1\}$
    \STATE Topologically order the executable subgraph induced by $S_\rho$
    \STATE Initialize staged successor map $Z\leftarrow\varnothing$
    \STATE Initialize temporary successor set $R_{\mathrm{tmp}}\leftarrow\varnothing$
    \STATE Initialize failure set $F_{\mathrm{tmp}}\leftarrow\varnothing$

    \FOR{each selected descendant $i\in S_\rho$ in topological order}
        \IF{$\bar P_i\not\subseteq \operatorname{dom}(Z)$}
            \STATE Add $i$ to $F_{\mathrm{tmp}}$ and keep $i$ withdrawn
        \ELSE
            \STATE Execute $\pi_i$ using $\mathsf{Ret}(e)$, $\kappa_e$, and staged predecessors
            $\{Z[j]\}_{j\in\bar P_i}$ to obtain successor $z_i$
            \IF{$\mathrm{Validate}_i(z_i)=1$}
                \STATE Set $Z[i]\leftarrow z_i$ and add $(i,z_i)$ to $R_{\mathrm{tmp}}$
            \ELSE
                \STATE Add $i$ to $F_{\mathrm{tmp}}$ and keep $i$ withdrawn
            \ENDIF
        \ENDIF
    \ENDFOR

    \FOR{each $i\in F_{\mathrm{tmp}}$}
        \STATE Set $v_i\leftarrow0$
    \ENDFOR
\UNTIL{$F_{\mathrm{tmp}}=\varnothing$}

\STATE Set $R_\rho\leftarrow R_{\mathrm{tmp}}$
\STATE Batch-republish all successors in $R_\rho$
\RETURN $(B_\rho,Q_\rho,S_\rho,R_\rho)$
\end{algorithmic}
\end{algorithm}

\subsection{Complexity and Scope}
\label{app:complexity-guarantees}

\textbf{Complexity.}
Cascade localization costs $O(|V|+|E^{\mathrm{inf}}|)$. Barrier broadcast has control-message cost $O(|\mathcal R_e|)$ over
reachable replicas, with payload $O(|\mathcal R_e||C(F)|)$ if hidden
artifact identifiers are transmitted explicitly. Instantiating local repair contracts
$\{\Psi_e(i):i\in D(F)\}$ costs $O(|D(F)|)$ excluding operator execution
time. Building $E^{\mathrm{req}}$ and detecting cyclic requirements costs
$O(|D^+(F)|+|E^{\mathrm{req}}|)$, or $O(|D^+(F)|^2)$ in the dense case.
With push--relabel, one min-cut call costs
\[
O(|Q_\rho|^3)\le O(|D^+(F)|^3).
\]
Each failed execution round marks at least one previously executable
candidate non-executable. The retry loop therefore runs at most
$|D^+(F)|$ times, giving worst-case selector-and-retry complexity
\[
O(|D^+(F)|^4),
\]
again excluding the cost of external repair operators such as LLM
regeneration, sandbox execution, or parameter-level repair.

\begin{assumption}[Monotone merge]
\label{asm:merge}
Each replica maintains grow-only sets $A$ (added), $B$ (hidden), and
$T$ (deleted). Merge is componentwise union, and visibility at replica
$r$ is
\[
\mathsf{Vis}_r(x)=\mathbf{1}[x\in A_r\setminus(B_r\cup T_r)].
\]
All updates are eventually delivered, and fenced replicas merge the
current barrier state before returning to service.
\end{assumption}

\begin{proposition}[Localization preservation under SCC condensation]
\label{prop:localization}
Let $\mathcal{G}_{\mathrm{raw}}$ be the raw durable-artifact influence
graph and let $\mathcal{G}_{\mathrm{cond}}$ be its SCC condensation. For
any root set $F$ and durable artifact $v$, $v$ is reachable from some
$f\in F$ in $\mathcal{G}_{\mathrm{raw}}$ if and only if the SCC
containing $v$ is reachable from some SCC containing a root in $F$ in
$\mathcal{G}_{\mathrm{cond}}$.
\end{proposition}

\begin{proof}[Proof]
Let \(G_{\mathrm{raw}}=(V_{\mathrm{raw}},E_{\mathrm{raw}})\) be the raw
durable-artifact influence graph, and let
\(G_{\mathrm{cond}}=(V_{\mathrm{cond}},E_{\mathrm{cond}})\) be its SCC
condensation. Write \(u\leadsto v\) if there exists a directed path
from \(u\) to \(v\) in \(G_{\mathrm{raw}}\), and let \([u]\) denote the
strongly connected component containing \(u\). For a root set
\(F\subseteq V_{\mathrm{raw}}\), define
\[
[F]\triangleq \{[f]:f\in F\}.
\]
By construction,
\[
V_{\mathrm{cond}}=\{[u]:u\in V_{\mathrm{raw}}\},
\]
and there is an edge \(([a],[b])\in E_{\mathrm{cond}}\) if and only if
\([a]\neq [b]\) and there exist \(u\in [a]\), \(v\in [b]\) such that
\((u,v)\in E_{\mathrm{raw}}\).

We must show that for any root set \(F\subseteq V_{\mathrm{raw}}\) and
any artifact \(v\in V_{\mathrm{raw}}\),
\[
\exists f\in F:\ f\leadsto v \text{ in } G_{\mathrm{raw}}
\quad\Longleftrightarrow\quad
\exists f\in F:\ [f]\leadsto [v] \text{ in } G_{\mathrm{cond}}.
\]

Assume first that there exists \(f\in F\) such that \(f\leadsto v\) in
\(G_{\mathrm{raw}}\). Then there is a directed path
\[
f=u_0\to u_1\to \cdots \to u_\ell=v.
\]
Projecting this path onto SCC labels gives
\[
[u_0],[u_1],\ldots,[u_\ell].
\]
After removing repeated consecutive labels, we obtain a sequence
\[
C_0,C_1,\ldots,C_m
\]
with \(C_0=[f]\), \(C_m=[v]\), and \(C_r\neq C_{r+1}\) for all \(r\).
For each transition \(C_r\to C_{r+1}\), there exists an edge
\((u_k,u_{k+1})\in E_{\mathrm{raw}}\) with \(u_k\in C_r\) and
\(u_{k+1}\in C_{r+1}\), hence
\((C_r,C_{r+1})\in E_{\mathrm{cond}}\). Therefore
\[
[f]=C_0\leadsto C_m=[v]
\]
in \(G_{\mathrm{cond}}\).

For the reverse direction, assume \([f]\leadsto [v]\) in
\(G_{\mathrm{cond}}\) for some \(f\in F\). Then there is a path
\[
[f]=C_0\to C_1\to \cdots \to C_m=[v]
\]
in \(G_{\mathrm{cond}}\).

If \(m=0\), then \([f]=[v]\), so \(f\) and \(v\) lie in the same SCC
and hence \(f\leadsto v\) in \(G_{\mathrm{raw}}\).

Now suppose \(m\ge 1\). By the definition of condensation edges, for
each \(r=0,\ldots,m-1\), there exist vertices \(a_r\in C_r\) and
\(b_r\in C_{r+1}\) such that
\[
(a_r,b_r)\in E_{\mathrm{raw}}.
\]
Because each \(C_r\) is strongly connected, any two vertices inside
\(C_r\) are mutually reachable. Hence inside \(C_0\) there is a path
from \(f\) to \(a_0\), inside each intermediate component \(C_r\) there
is a path from \(b_{r-1}\) to \(a_r\), and inside the final component
\(C_m=[v]\) there is a path from \(b_{m-1}\) to \(v\). Concatenating
these intra-SCC paths with the inter-SCC edges \((a_r,b_r)\) yields a
directed path from \(f\) to \(v\) in \(G_{\mathrm{raw}}\).

It follows that
\[
v\in C_{\mathrm{raw}}(F)
\quad\Longleftrightarrow\quad
[v]\in C_{\mathrm{cond}}([F]),
\]
where
\[
C_{\mathrm{raw}}(F)\triangleq
\{u\in V_{\mathrm{raw}}:\exists f\in F,\ f\leadsto u\},
\]
and
\[
C_{\mathrm{cond}}([F])\triangleq
\{C\in V_{\mathrm{cond}}:\exists f\in F,\ [f]\leadsto C\}.
\]
Equivalently,
\[
C_{\mathrm{raw}}(F)=\bigcup_{C\in C_{\mathrm{cond}}([F])} C.
\]
Therefore, SCC condensation preserves descendant localization exactly,
modulo replacing each SCC by its meta-node. This proves the
proposition.

\end{proof}

\begin{proposition}[Service-withdrawal isolation on reachable replicas]
\label{prop:isolation}
Under Assumption~\ref{asm:merge}, once an artifact enters $B$ or $T$ on
a reachable serving replica, no later merge makes that same artifact
visible again.
\end{proposition}

\begin{proof}[Proof]

Under Assumption~\ref{asm:merge}, each replica \(r\) maintains three
grow-only sets,
\[
A_r,\qquad B_r,\qquad T_r,
\]
where \(A_r\) is the set of added artifacts, \(B_r\) is the set of
hidden artifacts, and \(T_r\) is the set of deleted artifacts. Replica
merge is defined componentwise by set union: if the local state before
merge is \((A_r,B_r,T_r)\) and the incoming state is
\((A_{r'},B_{r'},T_{r'})\), then the post-merge state is
\[
A_r^{+}=A_r\cup A_{r'},\qquad
B_r^{+}=B_r\cup B_{r'},\qquad
T_r^{+}=T_r\cup T_{r'}.
\]
In particular, \(B_r\) and \(T_r\) are monotone: once an identifier
enters either set, it cannot be removed by any future merge.

Visibility at replica \(r\) is
\[
\mathsf{Vis}_r(x)=\mathbf{1}\!\left[x\in A_r\setminus(B_r\cup T_r)\right].
\]
Equivalently, \(\mathsf{Vis}_r(x)=1\) if and only if
\(x\in A_r\), \(x\notin B_r\), and \(x\notin T_r\).

Suppose that at some time an artifact \(x\) enters \(B_r\cup T_r\) on a
reachable replica \(r\). Since both \(B_r\) and \(T_r\) evolve only by
set union, every later local state and every later merged state still
satisfies
\[
x\in B_r\cup T_r.
\]
Hence
\[
\mathsf{Vis}_r(x)=0
\]
at that time and at all subsequent times. Therefore, once \(x\) is
hidden or deleted at replica \(r\), no future merge can make that same
artifact visible again on that replica.

At the beginning of repair event \(e\), the system computes
\[
B_\rho \leftarrow C(F)
\]
and propagates \(B_\rho\) to all reachable replicas. A reachable replica
acknowledges the barrier only after every artifact in \(B_\rho\) has
become non-servable locally. If a replica fails to acknowledge within
the timeout \(T_{\mathrm{ack}}\), it is fenced and removed from the
serving set until it reconnects and merges the current barrier state.
Consequently, every replica that remains reachable and allowed to serve
during the repair epoch satisfies
\[
C(F)=B_\rho\subseteq B_r.
\]
By the monotonicity proved above, every artifact \(x\in C(F)\) then
satisfies
\[
\mathsf{Vis}_r(x)=0
\]
throughout the repair interval on every reachable serving replica.

Thus, once an artifact enters \(B_r\) or \(T_r\) on a reachable
replica, no subsequent merge can make that same artifact visible again.
This does not preclude later publication of a validated fresh successor
version $z_i$ with a new artifact identifier; it only rules out
re-exposure of the original hidden or deleted artifact $x$ by merge.
\end{proof}

\textbf{Scope.}
The guarantees are store-level guarantees and require complete influence
provenance for cascade localization. For
$\mu_i\in\{\mathsf{recompute},\mathsf{regen}\}$, fresh successors are
constructed from retained valid support, staged repaired predecessors,
and the post-event interface $\kappa_e$. Recomputation applies only to
deterministic descendants. Regeneration produces validated successors
from retained support but does not claim exact causal subtraction. For
$\mu_i=\mathsf{param}$, exact parameter-level erasure is claimed only
when the chosen parameter-level repair operator provides such a
guarantee.

\newpage
\section{Broader Impact}
\label{sec:impact}

\textsc{MemoRepair} is designed to make persistent agent memories easier to keep current after deletions, corrections, or interface migrations. In systems that reuse summaries, cached tool outputs, procedures, or learned skills across sessions, it gives operators a clear way to identify affected descendants, take them out of service, rebuild valid successors, and republish only checked artifacts. This can improve reliability, reduce accidental reuse of outdated memory, and make memory updates easier to audit in deployed agentic systems. The same mechanism depends on accurate provenance and validation: missing influence edges or
incorrect checks can leave stale descendants unrepaired or republish faulty successors, so deployment
should keep audit logs and avoid treating store-level repair as a complete privacy or correctness guarantee.
